# Supplementary material for: Supervised Learning in the Presence of Noise: Application in ICD-10 Code Classification
Source: arXiv:2103.07808 source file (2021-03-13)
Supplement: Supplementary file 1 [file 99_Appendix.tex]

\appendix
