# Supplementary material for: Supervised Learning in the Presence of Noise: Application in ICD-10 Code Classification
Source: arXiv:2103.07808 source file (2021-03-13)
Supplement: Supplementary file 2 [file appendix_full_score_proposed.tex]

\begin{table*}[htbp]
\begin{tabular}{l|c|ccc|cc}
\toprule
\textbf{}               & \textbf{Vanilla} & \textbf{Modified label} & \textbf{Proposed} & \textbf{MLP + BR} & \textbf{Dev set trained} & \textbf{Dev set fine-tuned} \\ \hline
M54.5                   & 0.350            & 0.766                   & 0.795             & 0.395             & 0.069                    & 0.404                       \\
R10.9                   & 0.533            & 0.498                   & 0.501             & 0.386             & 0.068                    & 0.401                       \\
R92.8                   & 0.661            & 0.694                   & 0.687             & 0.620             & 0.635                    & 0.584                       \\
M54.2                   & 0.639            & 0.682                   & 0.682             & 0.633             & 0.150                    & 0.538                       \\
R53.1                   & 0.698            & 0.676                   & 0.733             & 0.732             & 0.016                    & 0.679                       \\
M25.561                 & 0.319            & 0.707                   & 0.627             & 0.656             & 0.052                    & 0.651                       \\
M25.562                 & 0.272            & 0.639                   & 0.621             & 0.566             & 0.013                    & 0.529                       \\
R10.2                   & 0.586            & 0.706                   & 0.758             & 0.645             & 0.192                    & 0.647                       \\
M25.511                 & 0.758            & 0.784                   & 0.958             & 0.533             & 0.017                    & 0.510                       \\
M79.671                 & 0.430            & 0.100                   & 0.171             & 0.107             & 0.015                    & 0.122                       \\
M54.6                   & 0.183            & 1.000                   & 1.000             & 0.833             & 0.003                    & 1.000                       \\
R11.2                   & 0.478            & 0.780                   & 0.765             & 0.766             & 0.026                    & 0.763                       \\
R55                     & 0.729            & 0.063                   & 0.063             & 0.063             & 0.010                    & 0.049                       \\
R41.0                   & 0.700            & 0.543                   & 0.545             & 0.608             & 0.004                    & 0.527                       \\
R10.13                  & 0.000            & 0.500                   & 0.500             & 1.000             & 0.009                    & 0.500                       \\
R09.89                  & 0.367            & 0.471                   & 0.722             & 0.710             & 0.009                    & 0.705                       \\ \hline
MAP & 0.481            & 0.600                   & 0.633             & 0.578             & 0.080                    & 0.538                 \\
\bottomrule
\end{tabular}
\caption{All AP for each of selected codes for all the methods on validated labels (full data for Table 6). }
\end{table*}
